# Supplementary material for: One-Loop Yukawa Corrections to the Process pp -> b anti-b H in the Standard Model at the LHC: Landau Singularities
Source: arXiv:0810.4078 source file (2008-11-14)
Supplement: Supplementary file 1 [file appendix_bbH_qcd.tex]

\chapter{The closed top loops}
\label{appendix-bbH-qcd}
\begin{figure}[h]
\begin{center}
\includegraphics[width=15cm]{psfig/ggbbH_qcd_top.eps}
\caption{\label{diag_qcd_top}{\em A generic set of QCD diagrams where the Higgs couples to a top loop.}}
\end{center}
\end{figure}

The purpose of this section is to point out that there exists a huge correction to the process 
$gg\to b\bar{b}H$. As pointed out in \cite{fawzi_bbH}, loop correction can bring an $\la_{bbH}$-independence 
contribution to this process. In order to calculate this contribution, we set $m_b=\la_{bbH}=0$. The only set of 
Feynman diagrams left is displayed in Fig. \ref{diag_qcd_top}. This group of diagrams 
is gauge invariant and ultraviolet finite.
It is obvious from those diagrams that the cross section is proportional to $g_s^8\la_t^2$. 
In order to avoid the colinear divergence occurring when 
a gluon splits into two massless bottom quarks, 
we have to impose an additional cut $M_{b\bar{b}}>20$GeV. Other kinematic cuts on the 
bottom transverse momenta and pseudo rapidities are kept the same as in the previous section.     
The EW and QCD cross sections are shown in Table. \ref{sigma_ew_qcd}. 
We can see that the QCD cross section is about $50$ times bigger than 
the EW one. 
The bulk of this big QCD correction originates in the diagrams containing the triangle $gg\to H$. 
If we look at the NLO QCD correction, i.e. the interference between the one-loop and the tree levels, 
the contribution of this class of top-quark loop diagrams only amount to about $-10\%$ of the NLO cross section \cite{dittmaier_bbH}. We can easily 
explain why this contribution is so small by looking at the helicity structures in the limit $m_b\to 0$: 
the dominant helicity configuration 
is even at the tree level and odd for the top-quark loop diagrams. 
This contribution vanishes when $m_b=0$. In this respect, we may expect a large 
correction by taking the square of these loop diagrams. 
Compared to the tree level cross section $\sigma_{LO}=0.02947$pb, 
the QCD correction in Table \ref{sigma_ew_qcd} is about $142\%$. This is the leading 
contribution in the $\la_{bbH}$ expansion. The $b\bar{b}$ invariant mass and $p_T^H$ distributions are shown in Fig. \ref{p_LLewqcd_mbb_pTH}.
\begin{table*}[t]
\caption{$\sqrt{s}=14$TeV, $M_H=120$GeV, $|\textbf{p}_{T}^{b,\bar{b}}|>20$GeV, $|\eta^{b,\bar{b}}|<2.5$, $M_{b\bar{b}}>20$GeV, $m_b=\la_{bbH}=0$.}
\begin{center}
\begin{tabular}{|c|c|c|c|}  \hline
$\sigma_{EW}[fb]$ &$\sigma_{QCD}[fb]$ &$\sigma_{(EW+QCD)}[fb]$ \\
\hline $0.8346(\pm 0.092\%)$ &$41.9864(\pm 0.079\%)$ &$43.773(\pm 0.076\%)$\\
\hline
\end{tabular}\label{sigma_ew_qcd}
\end{center}
\end{table*}
\begin{figure}[t]
\begin{center}
\begin{minipage}[t]{8.0cm}
\includegraphics[width=7.8cm]{psfig/p_LLewqcd_mbb_final.eps}
\end{minipage}
\begin{minipage}[t]{7.8cm}
\includegraphics[width=7.8cm]{psfig/p_LLewqcd_pTH_final.eps}
\end{minipage}
\caption{\label{p_LLewqcd_mbb_pTH}{\em The $M_{b\bar{b}}$(left) and $p_T^H$(right) distributions in the limit of vanishing bottom-Higgs Yukawa coupling. $Q=\mu=M_Z$.}}
\end{center}
\end{figure}
